# Supplementary material for: Can a Single Model Master Both Multi-turn Conversations and Tool Use? CoALM: A Unified Conversational Agentic Language Model
Source: arXiv:2502.08820 source file (2025-02-19)
Supplement: Supplementary file 1 [file appendix_main_results.tex]

\begin{table*}[!ht]
\centering
\resizebox{1.0\linewidth}{!}{
\begin{tabular}{l c c c c c c c c c c c c c c}
\toprule
\multirow{2}{*}{\textbf{Model}} & \multicolumn{2}{c}{Attraction} & \multicolumn{2}{c}{Hotel} & \multicolumn{2}{c}{Restaurant} & \multicolumn{2}{c}{Train} & \multicolumn{2}{c}{Taxi} & \multicolumn{3}{c}{\textbf{Total}} \\
		\cmidrule(lr){2-3}
		\cmidrule(lr){4-5}
		\cmidrule(lr){6-7}
		\cmidrule(lr){8-9}
            \cmidrule(lr){10-11}
  		\cmidrule(lr){12-14}
 & \textbf{Inform} & \textbf{Success} & \textbf{Inform} & \textbf{Success} & \textbf{Inform} & \textbf{Success} & \textbf{Inform} & \textbf{Success} & \textbf{Inform} & \textbf{Success} & \textbf{Inform} & \textbf{Success} & \textbf{BLEU} \\ \midrule

ReActTOD 8B (Mwoz)         & 65.6 & 37.1    & 61.4 & 32.0    & 78.7 & 45.8    & 83.8 & 41.3    & 100.0 & 19.5     & 58.5 & 29.7 & 14.0      \\ % 1e
%ReActTOD 8B C 3e         & 68.4 & 34.9    & 61.9 & 29.2    & 78.0 & 42.8    & 85.6 & 28.1    & 100.0 & 13.3     & 60.1 & 20.2 & 10.6      \\ % 3e
ReActTOD 8B (SGD-SNIPS)        & 62.8 & 36.7    & 70.6 & 49.5    & 86.5 & 50.1    & 81.2 & 58.9    & 100.0 & 40.0     & 63.4 & 43.1 & 10.7      \\ % 3e
ReActTOD 8B (Mwoz-SGD-SNIPS)       & 66.8 & 39.5    & 65.0 & 45.7    & 84.9 & 54.7    & 82.0 & 60.7    & 100.0 & 55.4     & 62.4 & 55.4 & 8.4      \\
ReActTOD 8B (Mwoz-MwozState-SGD-Hammer)       & 75.6 & 53.7    & 65.9 & 43.9    & 80.5 & 63.4    & 85.4 & 60.4    & 100.0 & 44.4     & \textbf{67.0} & \textbf{52.0} & 11.6      \\
ReActTOD 8B (Mwoz-SnipsState-SGD-Hammer-ToolAce)       & 63.4 & 36.6    & 62.7 & 45.1    & 89.2 & 51.4    & 85.4 & 52.1    & 100.0 & 42.9     & \textbf{57.0} & \textbf{46.0} & 11.6      \\\midrule % 3e
ToolACE-8B (100)         & 38.5 & 11.6    & 40.0 & 5.7     & 57.5 & 32.5    & 80.8 & 17.3    & 100.0 & 19.0     & 42.0 & 18.0 & 3.4      \\
Hammer-8B (100)          & 69.0 & 35.7    & 44.4 & 22.2    & 78.3 & 37.0    & 75.5 & 18.9    & 100.0 & 45.8     & 54.0 & 23.0 & 1.7      \\ \midrule

Llama 3.1 8B Instruct    & 53.9 & 35.4    & 58.4 & 21.3    & 70.3 & 34.3    & 82.8 & 25.1    & 100.0 & 0.0      & 49.8 & 19.9 & 1.74      \\
Mistral 7B Instruct      & 62.5 & 44.8    & 58.9 & 30.2    & 70.9 & 38.9    & 82.8 & 29.6    & 100.0 & 46.2     & 56.2 & 31.2 & 1.65      \\
Qwen2-7B-Instruct        & 79.2 & 62.8    & 71.8 & 55.8    & 90.8 & 63.4    & 85.0 & 67.0    & 100.0 & 69.2     & 71.6 & 60.7 & 3.50      \\ \midrule

Llama 3.1 405B Instruct  & 88.2 & 73.4    & 88.0 & 86.4    & 96.1 & 84.1    & 91.4 & 81.2    & 100.0 & 86.6     & \underline{88.0} & \underline{79.4} & 10.1       \\ 
GPT4-o Mini              & 80.5 & 72.3    & 89.6 & 75.1    & 92.4 & 72.3    & 90.5 & 77.1    & 100.0 & 70.3     & 81.1 & 69.9 & 8.9       \\
GPT4-o                   & 84.6 & 74.4    & 91.6 & 83.0    & 92.4 & 72.3    & 94.5 & 81.4    & 100.0 & 74.4     & 85.3 & 75.5 & 9.9       \\\bottomrule
%Qwen2-72B-Instruct      & --    & --        & --      & --    & --      & --        & --      & --     & --      & --      & --     \\ 
%Mistral-8B-Instruct     & --    & --        & --      & --    & --      & --        & --      & --     & --      & --      & --      \\
%Mistral-Large-Instruct  & --    & --        & --      & --    & --      & --        & --      & --     & --      & --      & --      \\ \midrule
%PPTOD                   & --    & --        & --      & --    & --      & --        & --      & --     & --      & --      & --      \\ 
%AutoTOD                 & --    & --        & --      & --    & --      & --        & --      & --     & --      & --      & --      \\ 
%FuncTOD                 & --    & --        & --      & --    & --      & --        & --      & --     & --      & --      & --      \\ \midrule

% ReActTOD 8B    & --    & --    & --    & --    & --    & -- & --    & --    & --    & --    & --    & --  & --    & --    & --       \\
% ReActTOD 70B   & --    & --    & --    & --    & --    & -- & --    & --    & --    & --    & --    & --  & --    & --    & --       \\
% ReActTOD 405B  & --    & --    & --    & --    & --    & -- & --    & --    & --    & --    & --    & --   & --    & --    & --      \\ \bottomrule
\end{tabular}
}
\caption{\textbf{Main Leaderboard}.}
\label{tab: main_results}
\end{table*}
